# Supplementary material for: BARD: Bridging AutoRegressive and Diffusion Vision-Language Models Via Highly Efficient Progressive Block Merging and Stage-Wise Distillation
Source: arXiv:2604.16514 source file (2026-07-12)
Supplement: Supplementary file 1 [file appendix.tex]

\section{Appendix}
